# Supplementary material for: Online Learning and Unlearning
Source: arXiv:2505.08557 source file (2025-05-13)
Supplement: Supplementary file 1 [file exact-unlearning.tex]

\subsection{exact unlearning}

Meta algorithm for exact unlearning 

Idea: keep a geometric covering interval \citep{daniely2015strongly} of the sequence, and when unlearning happens, restart with the longest sequence in the geometric covering interval that does not include the points to be unlearned. 

\includegraphics[width=0.5\textwidth]{AISTATS2025PaperPack/main_files/geometric.jpg}

For a set of strategies $W$, let $B$ be an algorithm whose regret with respect to $W$ satisfies \[R_B(T) \leq CT^\alpha\]for constants $C > 0$ and $\alpha \in (0, 1)$. 

Let $t_0 = 0$. Then the online learning unlearning algorithm $U$ through reweighting of a set of online learning algorithm based on $B$ has regret

\begin{align*}
    R_{U_B}(T) &\leq C(t_1)^\alpha + \sum_{i = 1}^{k-1} C\bs{\br{\frac{\Delta_i}{2} + t_{i + 1}}^\alpha - \br{\frac{\Delta_i}{2}}^\alpha}
\end{align*}
% where $\cT_i = \sum_{j = 1}^i t_j$. 
where $\Delta_i = t_i - t_{i-1}$. 

We note that the regret $R_{U_B}(T) \leq \sum_{i = 0}^{k-1}C (t_{i+1}-t_i)^\alpha$ for any $\cT$ but can be much smaller for some $\cT$. 

\begin{itemize}
    \item Time complexity for update at time step $t$: $O(\log t)$ $\sum_{t = 1}^T \log t \leq T\log T$
    \item Space complexity $O(2T)$. 
    \item Difference from adaptive learning: the learner knows points before the unlearning point are useful 
    \item We consider a local competitor defined by the largest geometric covering interval that does not include the unlearning points, so the online learner unlearner is robust to concept change. 
\end{itemize}
