# Supplementary material for: Online Learning and Unlearning
Source: arXiv:2505.08557 source file (2025-05-13)
Supplement: Supplementary file 2 [file exp_concave.tex]

\subsection{Exp-Concave loss}
\begin{defn}[$\alpha$-exp-concave function \cite{elad2019introduction}]
A convex function $f:\bR^d \to \bR$ is defined to be $\alpha$-exp concave over $\bR^d$ if the function $g(x) = e^{-\alpha f(x)}$ is concave. 
\end{defn}

Exp-concavity implies strong-convexity in the direction of gradient. 
\begin{lem}[\cite{elad2019introduction}]\label{lem:exp-concave}
A twice-differentiable function $f:\bR^n \to \bR$ is $\alpha$-exp-concave at $x$ if and only if \[\nabla^2 f(x)\succcurlyeq \alpha\nabla f(x)\nabla f(x)^\top.\]
\end{lem}

\begin{algorithm}
\caption{Input: learning rate $\eta_t$; diameter of the parameter space $D$; loss function $\ell_1, ..., \ell_T$ that are $L$-Lipschitz, $\gamma$-strongly convex, and $\beta$-smooth; contractive coefficient $\lambda$, deletion index and time set $\cJ, \cT$, unlearning parameter $\epsilon, \delta$}\label{alg:learning-unlearning-online-newton}
\begin{algorithmic}
\State Set $A_0 = \tau I$. 
\For{t = 1, 2, ..., }
\If{$t\notin \cT$ (i.e. only learning)}
\State Update \begin{equation}\label{eq:updating-rule-learning-newton}
\begin{aligned}
    A_t &= A_{t-1} + \nabla \ell_t(w_t) (\nabla \ell_t(w_t))^\top\\
    x_{t+1} &= \prod_{\cK}^{A_k} \br{x_t - \frac{1}{\gamma} A_t^{-1}\nabla \ell_t(w_t)}
\end{aligned}
\end{equation}
\ElsIf{$t\in \cT$, $t = t_i$ (i.e.unlearning and learning)}
% \State Set $\sigma_i = \br{\frac{\beta/\gamma - 1}{\beta/\gamma + 1}}^{t_i - j_i}LD/\epsilon$.
Set $\sigma_i = \lambda^{t_i - j_i}LD/\epsilon$.
\State Update \begin{align}\label{eq:update-rule-unlearning-newton}
    w_t &= w_t + \cN(0, \sigma_i^2)\\
    \tilde{w}_{t+1}&= \Pi_{\cW} (w_t - \eta_t \nabla \ell_t(w_t))
\end{align}
\EndIf
\EndFor
\end{algorithmic}
\end{algorithm}
% \RegretExpConcave*

\begin{proof}[Proof of~\Cref{thm:acc-exp-concave}]
    The first part of the proof follows by Lemma 4.6 in~\citet{elad2019introduction}, 
    \begin{lem}[Lemma 4.6 in~\citet{elad2019introduction}]
        \label{lem:exp-concave-regret}
        The regret of online Newton step is bounded by 
        \begin{equation}
            \text{Regret}_T(ONS)\leq \br{\frac{1}{\alpha} + LD}\br{\sum_{t = 1}^T\nabla_t^\top A_t^{-1} \nabla_t + 1}
        \end{equation}
    \end{lem}
    To upper bound the term $\sum_{t = 1}^T\nabla_t^\top A_t^{-1} \nabla_t$, let's define $A\bullet B = \sum_{i = 1}^d\sum_{j = 1}^d A_{ij}B_{ij} = Tr(AB^\top)$. Then
    \begin{equation}\label{eq:exp-concave-telescoping-sum}
        \begin{aligned}
         \sum_{t = 1}^T\nabla_t^\top A_t^{-1} \nabla_t &= \sum_{t = 1}^TA_t^{-1}\bullet \nabla_t\nabla_t^\top \\
        &= \sum_{t = 1}^T A_t^{-1}(A_t - A_{t-1})\\
        &\overset{(a)}{\leq} \sum_{i = 1}^T \log \frac{\abs{A_t}}{\abs{A_{t-1}}} = \log \frac{\abs{A_T}}{\abs{A_0}}
        \end{aligned}
    \end{equation}
    where (a) follows by Lemma 4.7 in~\citet{elad2019introduction}
    \begin{lem}[Lemma 4.7 in~\citet{elad2019introduction}]
    Let $A\succcurlyeq B$ be two positive definite matrices. Then, 
    \[A^{-1} \bullet (A-B) \leq \log \frac{\abs{A}}{\abs{B}}.\]
    \end{lem}
    Therefore, the expected regret is upper bounded by 
    \begin{equation}
        \label{eq:exp-concave-expected-regret-upper-bound}
        \bE\bs{\text{Regret}_T}\leq \br{\frac{1}{\alpha} + LD}\br{\bE\log \frac{\det\br{A_T}}{\det\br{A_0}} + 1} = \br{\frac{1}{\alpha} + LD}\br{\bE\br{\log \det\br{A_T}}- \log {\det\br{A_0}} + 1} 
    \end{equation}
    Then, it remains to upper bound $\bE\det (A_T)$. 
    We note that $\abs{A_0} = \epsilon^d$ and $A_T = \epsilon I_d + \sum_{i\notin \cT}\nabla_{t_i}\nabla_{t_i}^T + \sum_{i\in \cT}\nabla_{t_i}\nabla_{t_i}^T$. Let $B = \epsilon I + \sum_{i\notin \cT}\nabla_{t_i}\nabla_{t_i}^T $ and let $H = \sum_{i\in \cT}\nabla_{t_i}\nabla_{t_i}^T$. Then, 
    \begin{equation}\label{eq:exp-concave-log-det-upper-bound}
        \begin{aligned}
            \log \det (A_T) &= \log \det (B + H) \\
            &\overset{(a)}{\leq}\log \br{ \det(B) \det\br{I + \frac{H}{\lambda_{\min}(B)}}}\\
            &\overset{(b)}{\leq} \log \bs{\det(B)  \br{\frac{tr\br{I + \frac{H}{\lambda_{\min}(B)}}}{d}}^d }\\
            &= \log \br{\frac{\det (B) }{d^d} } + d \log 
            \bs{tr\br{I + \frac{H}{\lambda_{\min}(B)}}}
        \end{aligned}
    \end{equation}
    where step (a) follows from~\Cref{lem:upper-bound-determinant-of-sums} and step (b) follows from~\Cref{lem:determinant-trace-ineq}
    \begin{lem}
        \label{lem:upper-bound-determinant-of-sums}
        For any positive definite matrix $A$ and positive semi-definite matrix $B$, 
        \[\det (A+ B)\leq \det(A) \det \br{I + \frac{B}{\lambda_{\min}(A)}}.\]
    \end{lem}
    \begin{lem}
        \label{lem:determinant-trace-ineq}
        Let $A\in \bR^{d \times d}$ be a positive semi-definite matrix, then the following inequality holds, 
        \[\frac{tr(A)}{d}\geq \br{\det (A)}^{1/d}\]
    \end{lem}
    Following~\Cref{eq:exp-concave-log-det-upper-bound}, 
    \begin{equation}
        \label{eq:exp-concave-expected-log-det-upper-bound}
        \begin{aligned}
            \bE\log \det (A_T) &= \log \br{\frac{\det (B) }{d^d} } + d \bE \log 
            \bs{tr\br{I + \frac{H}{\lambda_{\min}(B)}}} \\
            &\overset{(a)}{\leq}\log \br{\frac{\det (B) }{d^d} } + d \log \bE
            \bs{tr\br{I + \frac{H}{\lambda_{\min}(B)}}} \\
            &= \log \br{\frac{\det (B) }{d^d} } + d \log \bE \br{d + \frac{1}{\lambda_{\min}(B)} \sum_{t_i \in \cT}tr(\nabla_{t_i}\nabla_{t_i}^\top)} \\
            &= \log \br{\frac{\det (B) }{d^d} } + d \log \br{d + \frac{1}{\lambda_{\min}(B)} \sum_{t_i \in \cT}\bE\norm{\nabla_{t_i}}^2} 
        \end{aligned}
    \end{equation}
    where step (a) is due to Jensen's inequality. 
    It remains to upper bound $\bE\norm{\nabla_{t_i}}^2$ for each time step in the deletion time set $t_i\in \cT$. We note that by the unlearning rule, $\nabla_{t_i} = \nabla \ell (w_{t} + \eta)$ where $\eta\sim \cN(0, \sigma_i^2)$. By smoothness of the loss function, i.e. lipschitzness of the gradient of the loss function, 
    \begin{equation}\label{eq:exp-concave-noise-norm-upper-bound}
    \begin{aligned}
            \bE\norm{\nabla_{t_i}}^2 &\leq 2\beta^2 (1+L) \sigma_i^2 = \frac{2\beta^2 L^2 (1+L) }{\varepsilon^2}
    \end{aligned}
    \end{equation}
    Substituting~\Cref{eq:exp-concave-noise-norm-upper-bound} into~\Cref{eq:exp-concave-expected-log-det-upper-bound} and substitute~\Cref{eq:exp-concave-expected-log-det-upper-bound} into~\Cref{eq:exp-concave-expected-regret-upper-bound}, we get \begin{equation}
        \begin{aligned}
            \bE\bs{\text{Regret}_T} &\leq \br{\frac{1}{\alpha} + LD} \br{1-\log \det (A_0) + \log \br{\frac{\det (B)}{d^d}} + d\br{\log \br{d + \frac{k\beta^2 L^2(1+L)}{\lambda_{\min}(B)\varepsilon^2}}}}\\
            &\overset{(a)}{\leq} \br{\frac{1}{\alpha} + LD} \br{1 -d \log \epsilon - d\log d + d \log (TL^2 + \epsilon) + d\log \br{d +  \frac{k\beta^2 L^2(1+L)}{\epsilon \varepsilon^2}}}\\
            &\overset{(b)}{\leq} \br{\frac{1}{\alpha} + LD} \br{1 + n\log \br{\frac{T}{d}} + d\log \br{d+\frac{k\beta^2 (1+L)}{ \varepsilon^2}}}
        \end{aligned}
    \end{equation}
    where step (a) is due to the definition of $B$ such that $\det(B) \leq TL^2 + \epsilon$ and $\lambda_{\min}(B) \geq \epsilon$ and $A_0 = \epsilon I$. Step (b) follows from $\log \br{\frac{TL^2 + \epsilon}{\epsilon d}} \leq \log (TL^2\gamma^2 D^2 + 1)\leq \log T/d$ for $\epsilon = 1/\gamma^2D^2$ and $\gamma = 1/2 \min(1/LD, \alpha)$. 
\end{proof}

\begin{proof}[Proof of~\Cref{lem:upper-bound-determinant-of-sums}]
    \begin{align*}
        \det(A + B) &= \det (A) \det (I + A^{-1}B) \\
        &= \det (A) \det (I + B^{1/2}A^{-1}B^{1/2})\\
        &\leq \det (A) \det \br{I + \frac{B}{\lambda_{\min}(A)}}
    \end{align*}
\end{proof}
\begin{proof}[Proof of~\Cref{lem:determinant-trace-ineq}]
    Denote the eigenvalues of $A$ by $\lambda_1, ..., \lambda_d$. As $A$ is positive semi-definite, $\lambda_i\geq 0$ for all $i\in [d]$. 

    Then, 
    \begin{equation*}
        \frac{tr(A)}{d} = \frac{\sum_{i = 1}^d\lambda_i}{d} \overset{(a)}{\geq} \br{\prod_{i = 1}^d \lambda_i}^{1/d} = \br{\det(A)}^{1/d}, 
    \end{equation*}
    where step (a) follows by AM-GM inequality. 
\end{proof}
