# Supplementary material for: Online Learning and Unlearning
Source: arXiv:2505.08557 source file (2025-05-13)
Supplement: Supplementary file 3 [file first_order.tex]

\begin{algorithm}[htbp]
    \caption{Active first-order online learner and unlearner}
    \label{alg:ERM-first-order}
    \begin{algorithmic}[1]
        \REQUIRE Cost functions $f_1, ..., f_T$ that are $L$-Lipschitz, learning rates $\eta_1, ..., \eta_T$, integers $\cI_1$ and $\cI_2$, contractive coefficient $\gamma$, a deletion time set $\cT$, a deletion index set $\cU$, and privacy parameter $\varepsilon$. 
        \STATE Initialize $z_1\in \cK$. 
        \FOR{Time step $t = 2, ... T$}
            \STATE Set $z_t = z_{t-1} - \eta_t \nabla f_{t-1}(z_{t-1})$
            \IF{there exists $t_i\in \cT$ such that $t = t_i$}
            \STATE Conduct $\cI_1$ steps of gradient descent with $f_{1:t_i}$ and $\cI_2$ steps of gradient descent with $f_{1:t_i}\setminus \{f_{u_i}\}$ with learning rate $1/i$ where $i$ is the number of gradient descent step ($i\in[\cI]$). 
            \STATE Let $\Delta_{t_i} = t_i - t_{i-1}$. 
            \STATE Set $z_t = z_t + \xi_i$, where $\xi_i \sim \cN(0, \sigma_i^2)$ for $\sigma_i = \frac{ L\br{\gamma^{\cI_1 + \cI_2}+1}}{\varepsilon\mu}\sqrt{\frac{2(1 + \log \Delta_{t_i})}{\Delta_{t_i}}} + \frac{2L\gamma^{\cI_2} }{\varepsilon\mu (\Delta_{t_i} + 1)}$.
        \ENDIF
        \STATE Output $z_t$ 
        \ENDFOR
    \end{algorithmic}
\end{algorithm}

In the following, we prove its unlearning guarantee.

% \begin{algorithm}
% \caption{First-order online learner and unlearner $\cR_{\cA}^{(1)}$}\label{alg:first-order-online-learner-unlearner}
% \begin{algorithmic}
% \State \textbf{Input}: learning rate $\eta_t$; diameter of the parameter space $D$; contractive coefficient $\gamma$ and Lipschitz coefficient $L$ of the cost functions, deletion index and time set $\cJ, \cT$, unlearning parameter $\varepsilon, \delta$. 
% \For{t = 1, 2, ..., }
% \If{$\ell_t = \perp$}
% \State Set $z_{t} = z_{t-1}$. 
% \Else
% \State Set $\tilde{z}_{t} = z_{t-1} - \eta_t \nabla \ell_t(z_{t-1})$; 
% \If{there exists $t_i \in \cT$ such that $t = t_i$}
% \State Iterate $z_t = z_t - \frac{2}{\mu + \beta} \sum_{i = t_{i-1}}^{t_i} \nabla f_i(z_t)$ for $\cI_1$ times. 
% \State Iterate $z_t = z_t - \frac{2}{\mu + \beta} \br{\sum_{i = t_{i-1}}^{t_i} \nabla f_i(z_t)} - \nabla f_{u_i}$ for $\cI_2$ times.
% \State Sample $\xi_i\sim \cN\br{0, \sigma_i^2}$, where $\sigma_i = \frac{j L\br{\gamma^{\cI_1 + \cI_2}+1}}{\varepsilon\mu}\sqrt{\frac{2(1 + \log \Delta_{t_j})}{\Delta_{t_j}}} + \frac{2L\gamma^{\cI_2} }{\varepsilon\mu (\Delta_{t_j} + 1)}$ for $\gamma = \frac{\beta/\mu - 1}{\beta/\mu + 1}$.
% \State $z_{t} = \tilde{z}_{t} + \xi_i$. 
% \Else 
% \State $z_{t} = \tilde{z}_{t}$. 
% \EndIf
% \State Output $z_{t}$
% \EndIf
% \EndFor
% \end{algorithmic}
% \end{algorithm}

% \FirstOrderUnlearning*
\begin{theorem}[Unlearning guarantee of first-order unlearning]
    % \label{thm:first-order-unlearning-guarantee}
    If the cost functions are $L$-Lipschitz, $\beta$-smooth and $\mu$-strongly convex and satisfy~\Cref{assump:assumption1}, then the algorithm $\cR_{\cA}^{(1)}$ is an $(\alpha, \varepsilon)$-online learner and unlearner.
\end{theorem}

\begin{proof}[Proof of unlearning guanratee in~\Cref{thm:first-order-unlearning-guarantee}]
    We use the same notation as in the proof of~\Cref{thm:active-guarantee-general}. Let \(\cF = \{f_1, \ldots, f_T\}\) be a set of cost functions, and define \(\cF' = \{f_1', \ldots, f_T'\}\) such that
    \[
    f_i' =
    \begin{cases}
    f_i & \text{if } i \notin \cT, \\
    \perp & \text{if } i \in \cT.
    \end{cases}
    \]
    Let \(g_i\) denote the gradient descent function on \(f_i\), that is,
    \[
    g_i(w) = w - \eta_i \nabla f_i(w).
    \]
    Similarly, define \(g_i'\) as the gradient descent function on \(f_i'\):
    \[
    g_i'(w) = w - \eta_i \nabla f_i'(w).
    \]
    For each \(j \in [k]\), let \(\psi_j\) and \(\psi_j'\) represent the composition of all gradient descent steps between two deletion steps using $\cF$ and $\cF'$ respectively:
    \[
    \psi_j(w) = g_{t_{j-1}+1} \circ \cdots \circ g_{t_j}(w),
    \quad \text{and} \quad
    \psi_j'(w) = g_{t_{j-1}+1}' \circ \cdots \circ g_{t_j}'(w).
    \]
    
    Additionally, let \(\psi_u^{(1)}\) denote the function that performs \(\cI_1\) steps of gradient descent using the entire history between two deletions, and let \(\psi_u^{(2)}\) denote the function that performs \(\cI_2\) steps of gradient descent on all functions between two deletions, excluding the deleted data point. We note that \(\psi_u^{(1)}\) depends on \(i\), the number of deletions so far; however, we omit this dependence for notation simplicity.

    Let $\zeta_j$ be the distribution of $\cN(0, \sigma_i^2I_d)$, where $\sigma_i $ as defined in~\Cref{alg:first-order}. We note that the outputs from the online learning and unlearning algorithm and from retraining from scratch (excluding deleted points) can be represented as two CNIs (\Cref{defn:CNI}):
    \[
    z_{t_1:t_k}
    \;=\;
    \mathrm{CNI}_T\{\,z_{t_0}, \{\psi_u^{(2)} \circ \psi_u^{(1)}\circ \psi_j\}_{j=1}^k, \{\zeta_j\}_{j=1}^k\},
    \quad
    z_{t_1:t_k}'
    \;=\;
    \mathrm{CNI}_T\{\,z_{t_0}, \{\psi_j'\}_{j=1}^k, \{\zeta_j\}_{j=1}^k\}.
    \]
    For each \(i \in [n]\), the unlearning functions \(\psi_u^{(1)}, \psi_u^{(2)}\) also takes as input all functions \(f_{t_{i-1}:t_i}\) (the functions between two deletions) and the deleted point \(f_{u_i}\). We omit these inputs from the notation in this proof.

    By the Data Processing Inequality (or post-processing property) of Rényi divergence \citep{mironov2017renyi}, if \(\rdp{z_{t_i}}{z_{t_i}'} \le \varepsilon\) for all \(i \in [k]\), then every intermediate step from \(t_i\) to \(t_{i+1}\) also satisfies \(\rdp{z_{t_i:t_{i+1}}}{z_{t_i:t_{i+1}}'} \le \varepsilon\). Next, we apply \Cref{lem:PAI} to show that \(\rdp{z_{t_i}}{z_{t_i}'} \le \varepsilon\) for all \(i \in [k]\). To do so, we first compute \(s_j\) and then assign the sequence \(a_j\) accordingly.

    \begin{equation}\label{eq:first-order-unlearning-0}
        \begin{aligned}
            s_j &= \max_{z\in \cK}\norm{\psi_u^{(1)}\circ \psi_u^{(2)} \circ \psi_j(z) - \psi_j'(z)}_2 \\
            &= \max_{z\in \cK}\norm{\psi_u^{(1)}\circ \psi_u^{(2)} \circ \psi_j(z) - w_{0, j}^\star + w_{0, j}^\star - \psi_j'(z)}_2 \\
            &\leq \underbrace{\max_{z\in \cK}\norm{\psi_u^{(1)}\circ \psi_u^{(2)} \circ \psi_j(z) - w_{0, j}^\star }}_{\text{Part A}} + \underbrace{\max_{z\in \cK}\norm{ w_{0, j}^\star - \psi_j'(z)}_2}_{\text{Part B}}
        \end{aligned}
    \end{equation}
    where $w_{0, j}^\star = \argmin_{z} \sum_{t = t_{j-1}}^{t_j} f_t'(z)$ is the ERM computed over the cost functions between time step $t_{j-1}$ and $t_j$ without the deleted point. Similarly, we define $w_{1, j}^\star =\argmin_{z} \sum_{t = t_{j-1}}^{t_j} f_t(z)$ as the ERM computed over all intermediate cost functions between the $j-1$th deletion and $j$th deletion. 
    
    Then, we apply~\Cref{lem:convergence-incremental-gd-shift-lr} to upper bound part B. 

    \begin{lem}[Convergence of incremental gradient descent]\label{lem:convergence-incremental-gd-shift-lr}
        Let $\cF$ be a set of cost functions satisfying~\Cref{assump:assumption1}. For a set of cost functions $f_1, ..., f_T\in \cF$, let $F = \sum_{i = 1}^T f_i$. Assume each function $f_i$ is $L$-Lipschitz and $\mu$-strongly convex. Let $z_1, ..., z_T$ be a series of points from OGD on the cost functions $f_i$, specifically, $z_{t+1} = z_t - \eta_t \nabla f_t(z_t)$ where $\eta_t = \frac{1}{\mu (t+k)}$ is the learning rate. Then, the following holds, 
        \[\norm{z_{T} - z^\star} \leq \sqrt{\frac{k}{T}\norm{z_1 - z^\star}^2 + \frac{L^2\log \frac{k + T}{k }}{\mu^2T}},  \]
        where $z^\star = \argmin_z F(z)$. 
    \end{lem}
    % \begin{lem}[Convergence of incremental gradient descent]\label{lem:convergence-incremental-gd}
    % Let $\cF$ be a set of cost functions satisfying~\Cref{assump:assumption1}. For a set of cost functions $f_1, ..., f_T\in \cF$, let $F = \sum_{i = 1}^T f_i$. Assume each function $f_i$ is $L$-Lipschitz and $\mu$-strongly convex. Let $z_1, ..., z_T$ be a series of points from gradient descent on the cost functions $f_i$, specifically, $z_{t+1} = z_t - \eta_t \nabla f_t(z_t)$ where $\eta_t = \frac{1}{\mu t}$ is the learning rate. Then, the following holds, 
    % \[\norm{z_{T} - z^\star} \leq \frac{L}{\mu}\sqrt{\frac{2\br{1+\log T}}{T}},  \]
    % where $z^\star = \argmin_z F(z)$. 
    % \end{lem}
    Part B is upper bounded by 
    \begin{equation}
        \label{eq:first-order-unlearning-partB}
        \max_{z\in \cK} \norm{w_{0, j}^\star - \psi_j'(z)}_2 \leq \sqrt{\frac{t_{j-1}D^2}{\Delta_{t_j}} + \frac{L^2\log \frac{t_j}{t_{j-1}}}{\mu^2\Delta_{t_j}}}. 
    \end{equation}
    where $\Delta_{t_j} = t_j - t_{j-1}$. 
    
    Then, we will upper bound part A. We first show that for any $z\in \cW$, 

    \begin{equation}\label{eq:first-order-partA-ineq}
        \begin{aligned}
            \norm{\psi_u^{(2)} \circ \psi_j(z) - w_{0, j}^\star} &\leq \norm{\psi_u^{(2)} \circ \psi_j(z) - w_{1, j}^\star} + \norm{w_{1, j}^\star - w_{0, j}^\star}\\
            & \overset{(a)}{\leq} \gamma^{\cI_1}\norm{\psi_j(z) - w_{1, j}^\star} + \frac{2L}{\mu( t_j -t_{j-1}+ 1)}\\
            &\overset{(b)}{\leq} \gamma^{\cI_1}\sqrt{\frac{t_{j-1}D^2}{\Delta_{t_j}} + \frac{L^2\log \frac{t_j}{t_{j-1}}}{\mu^2\Delta_{t_j}}} + \frac{2L}{\mu (t_j-t_{j-1} + 1)},
        \end{aligned}
    \end{equation}
    
    where $\gamma = \frac{\beta/\mu - 1}{\beta/\mu + 1}$, step (a) follows by application of~\Cref{lem:gd-convergence-sc-smooth} and stability of ERM (\Cref{lem:stability-erm-multiple-points}), and step (b) follows by~\Cref{lem:convergence-incremental-gd-shift-lr} (i.e. similar to~\Cref{eq:first-order-unlearning-partB}).

    \begin{lemL}[Convergence of gradient descent \cite{chen20lecture_notes}]
        \label{lem:gd-convergence-sc-smooth}
        If the loss function $\ell$ is $\mu$-strongly convex and $\beta$-smooth, then the output $w_t$ of $T$-step gradient descent on $S$ with learning rate $\eta = \frac{2}{\mu + \beta}$ and initialization $w_0$ satisfies \[\norm{w_t - w^\star}_2\leq \gamma^T \norm{w_0 -w^\star}_2,  \]
        where $\gamma = \frac{\beta/\mu - 1}{\beta/\mu + 1}$ and $w^\star = \textrm{arg}\min_w \sum_{x\in S}\ell(w, x)$ is the minimizer of the loss function $\ell$ on the dataset $S$. 
    \end{lemL}

    Applying~\Cref{lem:gd-convergence-sc-smooth} again, we obtain an upper bound on part A, 
    \begin{equation}\label{eq:first-order-unlearning-partA}
        \begin{aligned}
        \max_{z\in \cW}\norm{\psi_u^{(1)}\circ \psi_u^{(2)} \circ \psi_j(z) - w_{0, j}^\star } &\leq \gamma^{\cI_2}  \norm{\psi_u^{(2)} \circ \psi_j(z) - w_{0, j}^\star} \\
        &\overset{(a)}{\leq} \gamma^{\cI_1 + \cI_2}\sqrt{\frac{t_{j-1}D^2}{\Delta_{t_j}} + \frac{L^2\log \frac{t_j}{t_{j-1}}}{\mu^2\Delta_{t_j}}} + \frac{2L\gamma^{\cI_2} }{\mu (t_j -t_{j-1}+ 1)} 
        \end{aligned}
    \end{equation}
    where step (a) follows by substituting~\Cref{eq:first-order-partA-ineq}.  

    Substituting the upper bound on part A~(\Cref{eq:first-order-unlearning-partA}) and part B~(\Cref{eq:first-order-unlearning-partB}) into~\Cref{eq:first-order-unlearning-0}, we have 
    \[s_j\leq \br{\gamma^{\cI_1 + \cI_2} + 1}\sqrt{\frac{t_{j-1}D^2}{\Delta_{t_j}} + \frac{L^2\log \frac{t_j}{t_{j-1}}}{\mu^2\Delta_{t_j}}} + \frac{2L\gamma^{\cI_2} }{\mu \Delta_{t_j}} := a_j.\]
    
    By setting $a_i = s_i$, we note that 
    \[\sigma_j^2 = \frac{\alpha j^\omega \omega a_j^2}{2\br{\omega - 1}\varepsilon}.\]
    
    By~\Cref{lem:PAI}, 
    \begin{equation}\label{eq:first-order-unlearning-3}
            \rdp{z_{t_i}}{z_{t_i}'} \leq \sum_{j = 1}^i R_\alpha(\zeta_{j}, a_j)  = \sum_{j = 1}^i \frac{\alpha s_j^2}{2\sigma_j^2} \overset{(a)}{=}   \sum_{j = 1}^i \frac{\omega - 1}{\omega j^\omega}\varepsilon \overset{(b)} \leq \varepsilon
    \end{equation}
    where step (a) follows the definition of $\sigma_i^2$, and step (b) follows by~\Cref{lem:series-bounds}.
\end{proof}

\begin{proof}[Proof of~\Cref{lem:convergence-incremental-gd-shift-lr}]
    Since each component function $f_i$ is $\mu$-strongly convex, the function \( F \) is \( T\mu \)-strongly convex. Therefore, for any \( z_T \in \cK \),
    \begin{equation}
        \label{eq:incrementalGD-strong-convexity-ineq}
        \frac{T\mu}{2} \norm{ z_T - z^\star }_2^2 \leq F(z_T) - F(z^\star),
    \end{equation}
    where \( z^\star \) is the minimizer of \( F \).
    
    Then, we show that $F(z_T) - F(z^\star)$ is upper bounded. 
    \begin{equation}
        \begin{aligned}
            F(z_T) - F(z^\star) &= \sum_{t = 1}^T f_t(z_T) - \sum_{t = 1}^T f_t(z^\star) \\
            &\leq \underbrace{ \sum_{t = 1}^T f_t(z_T) - \sum_{t = 1}^T f_t(z_t) }_{A} +\underbrace{ \sum_{t = 1}^T f_t(z_t) - \sum_{t = 1}^T f_t(z^\star)}_{B} 
        \end{aligned}
    \end{equation}

    Note that Part B corresponds to the regret of the Online Gradient Descent (OGD) algorithm with learning rate \(\eta_t = \frac{1}{\mu(k + t)}\). Below, we derive the regret of OGD for strongly convex cost functions using a standard analysis.

    Following the OGD update rule~(\Cref{eq:ogd-defn}), we rearrange the equation
    \[
    \|z_t - z^\star\|^2 = \|z_{t-1} - \eta_{t-1} \nabla f_{t-1}(z_{t-1}) - z^\star\|^2
    \]
    to obtain
    \begin{equation}
        \label{eq:incremental-gd-convergence-regret-ineq}
        \nabla f_t(z_t)^\top (z_t - z^\star) = \frac{\|z_t - z^\star\|^2 - \|z_{t+1} - z^\star\|^2}{2\eta_t} + \frac{\eta_t \|\nabla f_t(z_t)\|^2}{2}.
    \end{equation}

    Then, the regret can be upper bounded as follows:
    \begin{equation}\label{eq:incremental-gd-upperbound-B}
        \begin{aligned}
            \sum_{t = 1}^T f_t(z_t) - f_t(z^\star) &\overset{(a)}{\leq} \sum_{t = 1}^T \nabla f_t(z_t)^\top (z_t - z^\star) - \frac{\mu \norm{z_t - z^\star}}{2}\\
            &\overset{(b)}{\leq}\sum_{t = 1}^T \frac{\norm{z_t - z^\star}^2 - \norm{z_{t+1} - z^\star}}{2\eta_t} + \frac{\eta_t\norm{\nabla f_t(z_t)}^2}{2} - \frac{\mu\norm{z_t - z^\star}^2}{2}\\
            &= \sum_{t = 1}^T \br{\frac{1}{\eta_t} - \frac{1}{\eta_{t-1}} - \mu}\frac{\norm{z_t - z^\star}^2}{2} + \frac{\eta_t\norm{\nabla f_t(z_t)}^2}{2} \\
            &=  \frac{k\mu}{2}\norm{z_1 - z^\star}^2 + \sum_{t = 1}^T \frac{L^2}{2\mu(k + t)} \overset{(c)}{=} \frac{k\mu}{2}\norm{z_1 - z^\star}^2 + \frac{L^2}{2\mu}\log \frac{k + T}{k}
        \end{aligned}
    \end{equation}
    where step (a) follows from the strong convexity of each component function $f_i$ and step (b) follows by substituting~\Cref{eq:incremental-gd-convergence-regret-ineq}. Step (c) follows from the inequality, 
    \[\sum_{t = 1}^T \frac{1}{k + t} \leq \int_{x = 0}^T\frac{dx}{x + k} = \log \frac{k + T}{k}.\]
    It remains to upper bound Part A. We claim that for each \( t \in [T] \), 
    
    \begin{equation}\label{eq:incrementalGD-2}
        f_t(z_T) - f_t(z_t) \leq -\sum_{j=t}^{T-1} \eta_j \br{\nabla f_t(z_j)}^\top \nabla f_j(z_j).
    \end{equation}
    Hence, we can upper bound part A by
    \begin{equation}\label{eq:incrementalGD-A}
        \sum_{t=1}^T f_t(z_T) - \sum_{t=1}^T f_t(z_t)
        \overset{(a)}{\leq} -\sum_{t = 1}^T\sum_{j=t}^{T-1} \eta_j \br{\nabla f_t(z_j)}^\top \nabla f_j(z_j) \overset{(b)}{\leq} 0
    \end{equation}
    where step (a) follows from~\Cref{eq:incrementalGD-2} and step (b) follows from~\Cref{assump:assumption1}. 

    Combining the upper bound on Part A~(\Cref{eq:incrementalGD-A}) with the upper bound on Part B~(\Cref{eq:incremental-gd-upperbound-B}), and substituting this combined upper bound into~\Cref{eq:incrementalGD-strong-convexity-ineq}, we complete the proof.
    
    Next, we demonstrate that the claim in~\Cref{eq:incrementalGD-2} holds. For any \( t \in [T] \), using convexity and the definition of \( z_{1:T} \) following the update rule of OGD, i.e. $z_t = z_{t-1} - \eta_{t-1}\nabla f_{t-1}(z_{t-1})$, we have
    \begin{equation}\label{eq:incrementalGD-3}
        \begin{aligned}
            f_t(z_T) -f_t(z_{T-1})&\leq  - \eta_{T-1}\br{\nabla f_t(z_{T-1})}^\top \nabla f_{T-1}(z_{T-1})\\
            f_t(z_{T-1}) - f_t(z_{T-2}) &\leq  - \eta_{T-2}\br{\nabla f_t(z_{T-2})}^\top \nabla f_{T-2}(z_{T-2})\\
            & \ldots \\
            f_t(z_{t+1}) - f(z_t) &\leq  - \eta_{t}\br{\nabla f_t(z_{t})}^\top \nabla f_{t}(z_{t})
        \end{aligned}
    \end{equation}
    Summing all the inequalities in~\Cref{eq:incrementalGD-3}, we have \[f_t(z_T) -f(z_t) \leq -\sum_{j = t}^{T-1} \eta_{j}\br{\nabla f_t(z_{j})}^\top \nabla f_{j}(z_{j}). \]
\end{proof}

\begin{theorem}[Regret guarantee of first-order unlearning]
    Assume all loss functions are $L$-Lipschitz, $\mu$-strongly convex, $\beta$-smooth, and satisfy~\Cref{assump:assumption1}. Assume the set of deletion time $\cT$ satisfies $t_1 \geq \frac{2}{\mu}\sqrt{\varepsilon}L$ and $t_i \geq t_{i-1} + e^{D t_{i-1}}$ for all $i\in [k]$. Assume the index of the unlearning point $u_i \in (t_{i-1}, t_i)$ for all $i$. Then we can upper bound the regret of~\Cref{alg:first-order} by \[\bE\text{Regret}_T \leq \frac{L^2}{\mu}\br{2 + k(1 + k) +2\log T} + \sum_{i = 1}^k \frac{9t_i\br{\frac{\varepsilon}{i} + 2}L^2\br{\gamma^{\cI_1 + \cI_2} + 1}^2\log \Delta_{t_i}}{\mu\Delta_{t_i}}.\]
\end{theorem}

\begin{proof} 
    For a set of cost functions $\ell_1, \ldots, \ell_T$, where $\ell_{u_i} = \perp$ for all $i \in [k]$, we denote the best-in-hindsight estimator by $z^\star = \arg\min_{z \in \cW} \sum_{t=1}^{T-k} \ell_t(z)$. Recall that $\cT = \{t_1, ..., t_i\}$ is the set of deletion times. By the updating rule of~\Cref{alg:first-order}, for $t\notin \cT$, 
    
    \begin{equation}\label{eq:strongly-convex-first-order1}
        \begin{aligned}
        \norm{z_{t} - z^\star}^2 &= \norm{z_{t-1} - \eta_{t-1}\nabla\ell_{t-1}(z_{t-1}) - z^\star}^2\\
        &=\norm{z_{t-1} - z^\star }^2 + \eta_{t-1}^2\norm{\nabla \ell_{t-1}(z_{t-1})}^2 - 2\eta_{t-1} (\nabla\ell_{t-1}(z_{t-1}))^\top \br{z_{t-1} - z^\star}.
        \end{aligned}
    \end{equation}

    We recall that for each unlearning request, our unlearning algorithm starts from the current output $\hat{z}_t = z_{t-1} - \eta_{t-1} \nabla f_{t-1}(\hat{z}_t)$, which is obtained by performing one additional gradient descent step on the new cost function using the previous output. The algorithm first performs $\cI_1$ gradient descent steps with intermediate cost functions between the current and last deletion, followed by $\cI_2$ gradient descent steps with the same set of cost functions excluding the deleted one. For simplicity, we represent these gradient descent steps as a deterministic function $\FirstUn{i}$ for the $i^{\mathrm{th}}$ deletion. Finally, the unlearning algorithm adds noise $\xi_i$ to $\FirstUn{i}(\hat{z}_t)$ and outputs $z_t = \xi_i + \FirstUn{i}(\hat{z}_t)$.

    Then, for each $i\in [k]$, we write $\tilde{d}_i = z_t - \hat{z}_t$ and $d_i = z_t - \hat{z}_t + \xi_i$. For each $t\in \cT$, we have

    \begin{equation}\label{eq:strongly-convex-first-order2}
        \begin{aligned}
        \norm{z_t - z^\star}^2 &= \norm{d_i' + \hat{z_t} - z^\star}^2\\
        &\overset{(a)}{=} \norm{d_i' + z_{t-1} - \eta_{t-1}\nabla \ell_{t-1}(z_{t-1}) - z^\star}^2\\
        &= \bs{d_i' + \eta_{t-1}\nabla \ell_{t-1}(z_{t-1})}^2 + 2\br{d_i' - \eta_{t-1}\nabla \ell_{t-1}(z_{t-1})}^\top \br{z_{t-1}-z^\star}+ \norm{z_{t-1} - z^\star}^2\\
        \end{aligned}
    \end{equation}
    where step (a) follows the definition of $\hat{z}_t$ and definition of $d_i'$. 

    Rearrange~\Cref{eq:strongly-convex-first-order1} and~\Cref{eq:strongly-convex-first-order2}we have 
    \begin{equation}\label{eq:strongly-convex-first-order3}
    (\nabla\ell_{t}(z_{t}))^\top \br{z_{t} - z^\star} =\begin{cases} 
      \frac{\norm{z_{t}-z^\star}^2 - \norm{z_{t+1}-z^\star}^2}{2\eta_{t}} + \frac{\eta_{t}\norm{\nabla \ell_{t}(z_{t})}^2}{2} & t+1 \notin \cT \\
    \frac{\norm{z_{t}-z^\star}^2 - \norm{z_{t + 1}-z^\star}^2}{2\eta_{t}} + \frac{\br{d_i' + \eta_t \nabla \ell_t (z_t)}^2 + 2d_i'\br{z_t - z^\star}}{2\eta_{t}} &  t +1 = t_i\in\cT 
    \end{cases}
    \end{equation}

    By the definition of strong convexity of loss function $\ell_t$ (\Cref{defn:Lipschitzness-smoothness}), for all $t$, \[\ell_t(z_t) - \ell_t(z^\star) \leq \br{\nabla \ell_t (z_t)}^\top \br{z_t - z^\star} - \frac{\mu}{2}\norm{z_t - z^\star}^2.\]

    Summing over $t\in [T]$ and substitute~\Cref{eq:strongly-convex-first-order3} into the equation, 
    \begin{equation*}
        \begin{aligned}
            \sum_{t = 1}^T \ell_t(z_t) - \ell_t(z^\star) &= \sum_{t = 1}^T\br{\nabla \ell_t(z_t)}^\top (z_t - z^\star) - \frac{\mu}{2}\norm{z_t - z^\star} \\
            &= \underbrace{\sum_{t = 1}^T  \frac{\norm{z_{t}-z^\star}^2 - \norm{z_{t+1}-z^\star}^2}{2\eta_{t}} + \frac{\eta_{t}\norm{\nabla \ell_{t}(z_{t})}^2}{2} - \frac{\mu}{2}\norm{z_t - z^\star}}_{A} \\
            & + \underbrace{\sum_{i = 1}^k d_i'\nabla \ell_t(z_t) + \frac{d_i' \br{z_t - z^\star} + \br{d_i'}^2}{2\eta_t}}_{B}
        \end{aligned}
    \end{equation*}

    For simplicity, we write $A = \sum_{t = 1}^T  \frac{\norm{z_{t-1}-z^\star}^2 - \norm{z_{t}-z^\star}^2}{2\eta_{t-1}} + \frac{\eta_{t-1}\norm{\nabla \ell_{t-1}(z_{t-1})}^2}{2} + \frac{\gamma}{2}\norm{z_t - z^\star}$ and $B = \sum_{i = 1}^k d_i'\nabla \ell_t(z_t) + \frac{d_i' \br{z_t - z^\star} + \br{d_i'}^2}{2\eta_t}$. Then, the expected regret can be upper bounded as 
    \begin{equation}\label{eq:strongly-convex-first-order4}
        \begin{aligned}
            \bE\bs{\regret{T}{\cR_{\cA}}(S_T, \emptyset, \cT)}&= \bE_{\xi_{1:k}}\bs{A + B }\\
            &= \bE_{\xi_{1:k}}\bE\bs{A|\xi_{1:k}} + \bE_{\xi_{1:k}}\bs{B}
        \end{aligned}
    \end{equation}

    We first bound the first term $\bE\bs{A|\xi_{1:k}}$. Given $\xi_{1:k}$, $z_1, ..., z_T$ are deterministic. We set $\eta_t = \frac{1}{\mu t}$ and $1/\eta_0 = 0$, 
    \begin{equation*}
        \begin{aligned}
            \bE\bs{A|\xi_{1:k}} &= \sum_{t = 1}^T  \frac{\norm{z_{t}-z^\star}^2 - \norm{z_{t+1}-z^\star}^2}{2\eta_{t}} + \frac{\eta_{t}\norm{\nabla \ell_{t}(z_{t})}^2}{2} -\frac{\mu}{2}\norm{z_t - z^\star} \\
            &= \bE\bs{\sum_{t = 1}^T \br{\frac{1}{\eta_t}-\frac{1}{\eta_{t-1}}-\mu}\norm{z_t - z^\star}^2 + \sum_{t = 1}^T \frac{\eta_t \norm{\nabla \ell_t(z_t)}^2}{2}}\\
            &\overset{(a)}{=} \sum_{t = 1}\frac{\norm{\nabla\ell_t(z_t)}^2}{2\mu t} \overset{(b)}{\leq} \frac{L^2}{\mu}\br{1 + \log T}
        \end{aligned}
    \end{equation*}
    where step (a) is due to the definition of $\eta$, i.e. $\frac{1}{\eta_t}-\frac{1}{\eta_{t-1}}-\mu = 0$, and step (b) is due to the Lipschitzness of the cost function $\ell_t$ and that $\sum_{t = 1}^T \frac{1}{t}\leq 1 + \log T$. 

    Thus, 
    \begin{equation}\label{eq:strongly-convex-first-order5}
        \bE_{\xi_{1:k}}\bs{A} = \bE_{\xi_{1:k}} \bE\bs{A|\xi_{1:k}} \leq \frac{L}{\mu}(1 + \log T)
    \end{equation}

    It remains to bound $\bE_{\xi_{1:k}}\bs{B}$. We first note that $d_i' = d_i + \xi_i$ by our definition of $d_i'$ and $d_i$, 

    \begin{equation}\label{eq:strongly-convex-first-order6}
        \begin{aligned}
            \bE_{\xi_{1:k}}\bs{B} &\leq \sum_{i = 1}^k \bE_{\xi_{1:k}}\bs{(d_i + \xi_i)L + \frac{2(d_i + \xi_i)D + (d_i + \xi_i)^2}{2\eta_{t_i-1}}}\\
            &\overset{(a)}{\leq} \sum_{i = 1}^k\bE_{\xi_{1:k}}\bs{(d_i + \xi_i)L + \mu t_i \br{D + \frac{(d_i + \xi_i)^2}{2}}}\\
            &\overset{(b)}{=} d_i (L + \mu t_i  D) + \frac{\mu t_i (d_i^2 + \sigma_i^2)}{2}
        \end{aligned}   
    \end{equation}
    where step (a) follows by substituting in the learning rate $\eta_t = \frac{1}{\mu t}$ and step (b) is due to  $\bE\xi_i = 0$.

    Next, by an argument similar to~\Cref{eq:first-order-unlearning-0}, we can show that $d_i\leq \sigma_i\sqrt{\frac{\varepsilon}{i}}$, we obtained the final bound on 
    \begin{equation}
        \label{eq:first-order-regret-partB}
            \bE\bs{B}\leq\sum_{i = 1}^k \sqrt{\frac{\varepsilon}{i} }\sigma_i(L + \mu t_i D) + \frac{\mu t_i}{2} \br{\frac{\varepsilon}{i} + 1}\sigma_i^2
    \end{equation}
    By simple algebra, one can show that for all $i \in [k]$, \begin{equation}
        \label{eq:bounds-on-sigma2}
        \sigma_i^2 \leq \frac{i^2 L^2\br{\gamma^{\cI_1 + \cI_2} + 1}^2}{\varepsilon\mu^2}\frac{12\log \Delta_{t_i} + 3t_{i-1}D}{\Delta_{t_i}}
    \end{equation}

    \Todo{With application of~\Cref{lem:convergence-incremental-gd-shift-lr,lem:stability-erm-multiple-points} (specify $\norm{z_{t_{i-1}}-z^\star}$ term by decomposing it as approximation error of OGD to $ERM_1$ and the difference between two ERM solutions) , we can show that \[d_i \leq \sqrt{\frac{2D + \frac{L^2\log (T + k)/k}{\mu }}{T}}.\]}

    Therefore, substituting~\Cref{eq:bounds-on-sigma2} into~\Cref{eq:first-order-regret-partB}, we can upper bound $\bE\bs{B}$ by 
    \begin{equation}
        \label{eq:first-order-regret-partB-final}
        \begin{aligned}
            \bE\bs{B}&\overset{(a)}{\leq} \sum_{i = 1}^k \br{\sqrt{\frac{\varepsilon}{i}}L + \frac{\mu t_i}{2}\br{\frac{\varepsilon}{i} + 1}}\max\br{1, \sigma_i^2}
            \\&\leq \sum_{i = 1}^k \br{\sqrt{\frac{\varepsilon}{i}}L + \frac{\mu t_i}{2}\br{\frac{\varepsilon}{i} + 1}}\frac{L^2\br{\gamma^{\cI_1 + \cI_2} + 1}^2 i^2\br{12 \log \Delta_{t_i} + 3t_{i-1}D}}{\varepsilon\mu^2 \Delta_{t_i}},
        \end{aligned}
    \end{equation}
    where step (a) is due to the fact that for $\sigma_i \geq 1$, $\sigma_i \leq \sigma_i^2$. 

    Combining~\Cref{eq:strongly-convex-first-order4,eq:strongly-convex-first-order5,eq:first-order-regret-partB-final}, we have 
    \begin{equation}\label{eq:strongly-convex-first-order-final1}
        \bE\bs{\regret{T}{\cR_{\cA}\br{S_T, \emptyset, \cT}}} = \frac{L^2}{\mu}\br{1 + \log T} + \sum_{i = 1}^k \frac{9t_i\br{\frac{\varepsilon}{i} + 2}L^2\br{\gamma^{\cI_1 + \cI_2} + 1}^2\log \Delta_{t_i}}{\mu\Delta_{t_i}}
    \end{equation}

    In the following, we prove~\Cref{eq:bounds-on-sigma2}. 

    Recall that 
    \[\sigma_i^2 = \frac{L^2\br{\gamma^{\cI_1 + \cI_2} + 1}^2}{\mu^2}\frac{4\log \Delta_{t_j} + t_{j-1}D}{\Delta_{t_j}}  + \frac{4L^2\gamma^{2\cI_2}}{\mu^2\Delta_{t_j}^2} + \frac{2L^2\gamma^{\cI_2}\br{\gamma^{\cI_1 + \cI_2} + 1} }{\mu^2\Delta_{t_j}} \sqrt{\frac{4\log \Delta_{t_j} + t_{j-1}D}{\Delta_{t_j}}} 
    \]
    % \begin{equation}\label{eq:bounds-on-sigma2-1}
    %     \begin{aligned}
    %         \sigma_i^2 &= \frac{L^2\br{\gamma^{\cI_1 + \cI_2} + 1}^2}{\mu^2}\frac{4\log \Delta_{t_j} + t_{j-1}D}{\Delta_{t_j}}  + \frac{4L^2\gamma^{2\cI_2}}{\mu^2\Delta_{t_j}^2} + \frac{2L^2\gamma^{\cI_2}}{\mu^2\Delta_{t_j}} \br{\gamma^{\cI_1 + \cI_2} + 1} \sqrt{\frac{4\log \Delta_{t_j} + t_{j-1}D}{\Delta_{t_j}}}\\
    %         &\overset{(a)}{\leq}\frac{L^2\br{\gamma^{\cI_1 + \cI_2} + 1}^2}{\mu^2}\frac{5\log \Delta_{t_j}}{\Delta_{t_j}} + \frac{4L^2\gamma^{2\cI_2}}{\mu^2\Delta_{t_j}^2} + \frac{2L^2\gamma^{\cI_2}}{\mu^2\Delta_{t_j}} \br{\gamma^{\cI_1 + \cI_2} + 1} \sqrt{\frac{5\log \Delta_{t_j}}{\Delta_{t_j}}}
    %     \end{aligned}
    % \end{equation}
    % where step (a) follows by the fact that $\log \Delta_{t_j}\geq D t_{j-1}$ due to the assumption $t_i \geq t_{i-1} + e^{D t_{i-1}}$. 

    Next, as $\gamma^{2\cI_2}\leq 1$, we have 
    \begin{equation}
        \label{eq:sigma2-2}
        \frac{4L^2\gamma^{2\cI_2}}{\mu^2\Delta_{t_j}^2}\leq \frac{L^2\br{\gamma^{\cI_1 + \cI_2} + 1}^2}{\mu^2}\frac{4\log \Delta_{t_j}}{\Delta_{t_j}}
    \end{equation} 

    Similarly, one can easily show that \begin{equation}
        \label{eq:sigma2-3}
        \frac{2L^2\gamma^{\cI_2}}{\mu^2\Delta_{t_j}} \br{\gamma^{\cI_1 + \cI_2} + 1} \sqrt{\frac{5\log \Delta_{t_j}}{\Delta_{t_j}}} \leq \frac{L^2\br{\gamma^{\cI_1 + \cI_2} + 1}^2}{\mu^2}\frac{5\log \Delta_{t_j}}{\Delta_{t_j}}
    \end{equation}

    Combining these inequality, we get the desired bound on $\sigma_i^2$ (\Cref{eq:bounds-on-sigma2}). 

    Next, we bound the distance between $ \bE\bs{\regret{T}{R_{\cA}(S, \emptyset, \cT) }}$ and $ \bE\bs{\regret{T}{\cR_{\cA}(S, S_U, \cT)}}$ by definition of the regret with unlearning~(\Cref{eq:regret-defn}). 

    \begin{equation}\label{eq:strongly-convex-first-order-final2}
    \begin{aligned}
        \norm{\bE\bs{\regret{T}{\cR_{\cA}(S, \emptyset, \cT) }} - \bE\bs{\regret{T}{\cR_{\cA}(S,  S_U, \cT) }}} &=  \norm{\sum_{i = 1}^k \sum_{t = t_{i-1}}^{t_i} f_t(w^\star) - f_t(w_i^\star)}\\
        &\leq \sum_{i = 1}^k \sum_{t = t_{i-1}}^{t_i} L\norm{w^\star - w_i^\star}\\
        &\overset{(a)}{\leq} \sum_{i = 1}^k \sum_{t = t_{i-1}}^{t_i} L\frac{2Li}{\mu T} = \frac{(1 + k) k L^2}{\mu},
    \end{aligned}
    \end{equation}
    where step (a) follows~\Cref{lem:stability-erm-multiple-points}. 

    Combining~\Cref{eq:strongly-convex-first-order-final1,eq:strongly-convex-first-order-final2} concludes the proof. 
\end{proof}
