# Supplementary material for: Online Learning and Unlearning
Source: arXiv:2505.08557 source file (2025-05-13)
Supplement: Supplementary file 4 [file second_order.tex]

\begin{algorithm}
    \label{alg:ERM-second-order}
\end{algorithm}

% \begin{algorithm}
% \caption{Second-order online learner and unlearner $\cR_{\cA}^{(2)}$}\label{alg:second-order-online-learner-unlearner}
% \begin{algorithmic}
% \State \textbf{Input}: learning rate $\eta_t$; diameter of the parameter space $D$; contractive coefficient $\gamma$ and Lipschitz coefficient $L$ of the cost functions, deletion index and time set $\cJ, \cT$, unlearning parameter $\varepsilon, \delta$. 
% \For{t = 1, 2, ..., }
% \If{$\ell_t = \perp$}
% \State Set $z_{t} = z_{t-1}$. 
% \Else
% \State Set $\tilde{z}_{t} = z_{t-1} - \eta_t \nabla \ell_t(z_{t-1})$; 
% \If{there exists $t_i \in \cT$ such that $t = t_i$}
% \State Compute $H_i(z_t) = \sum_{t = t_{i-1}}^{t_i}\nabla^2f_t(z_t) - f_{u_i}(w)$. 
% \State Compute $z_t = z_t + \br{H_i(z_t)}^{-1}\nabla f_{u_i}$.
% \State Let $\gamma = \frac{\beta/\mu - 1}{\beta/\mu + 1}$ and $\Delta_i = t_i - t_{i-1}$.
% \State Sample $\xi_i\sim \cN\br{0, \sigma_i^2}$, where $\sigma_i = \frac{j L\br{\gamma^{\cI_1 + \cI_2}+1}}{\varepsilon\mu}\sqrt{\frac{2(1 + \log \Delta_{t_i})}{\Delta_{t_i}}} + \frac{2L\gamma^{\cI_2} }{\varepsilon\mu (\Delta_{t_i} + 1)}$. 
% \State $z_{t} = \tilde{z}_{t} + \xi_i$. 
% \Else 
% \State $z_{t} = \tilde{z}_{t}$. 
% \EndIf
% \State Output $z_{t}$
% \EndIf
% \EndFor
% \end{algorithmic}
% \end{algorithm}

\begin{theorem*}
    % \label{thm:first-order-unlearning-guarantee}
    If the cost functions are $L$-Lipschitz, $\beta$-smooth and $\mu$-strongly convex and satisfy~\Cref{assump:assumption1}, then the algorithm $\cR_{\cA}^{(2)}$ is an $(\alpha, \varepsilon)$-online learner and unlearner.
\end{theorem*}

\begin{proof}
    We use the same notation of $\cF, \cF'$, $g_i, g_i'$, $\psi_j$ and $\psi_j'$ as in the proof of~\Cref{thm:first-order-unlearning-guarantee}. For $j\in [k]$, let $\psi_u^{(j)}$ denote the $j$th unlearning function using second order information. Specifically, \[\psi_u^{(j)}(w) =  w + \br{H_j(w)}^{-1}\nabla f_{u_j}(w), \]
where $H_j(w) = \sum_{t = t_{j-1}}^{t_j}\nabla^2f_t(w) - f_{u_j}(w)$. 

Similarly, we rewrite the online learning and unlearning algorithm as two CNIs, \[\{z_{t_0}, \{\psi_u^{(j)}\circ\psi_j\}_{j = 1}^k, \{\zeta_j\}_{j = 1}^k\}, \quad \{z_{t_0}, \{\psi_j'\}_{j = 1}^k, \{\zeta_j\}_{j = 1}^k\}.\]

Applying~\Cref{lem:PAI}, we can show that $\rdp{z_{t_i}}{z_{t_i}'}\leq \varepsilon$ for all $i\in [k]$. We will derive the expression of $s_j$. 

\begin{equation}\label{eq:second-order-unlearning-0}
        \begin{aligned}
            s_j &= \max_{z\in \cW}\norm{\psi_u^{(j)} \circ \psi_j(z) - \psi_j'(z)}_2 \\
            &= \max_{z\in \cW}\norm{ \psi_u^{(j)} \circ \psi_j(z) - w_{0, j}^\star + w_{0, j}^\star - \psi_j'(z)}_2 \\
            &\leq \underbrace{\max_{z\in \cW}\norm{\psi_u^{(j)} \circ \psi_j(z) - w_{0, j}^\star }}_{\text{Part A}} + \underbrace{\max_{z\in \cW}\norm{ w_{0, j}^\star - \psi_j'(z)}_2}_{\text{Part B}}
        \end{aligned}
    \end{equation}
where $w_{0, j}^\star = \argmin_{z} \sum_{t = t_{j-1}}^{t_j} f_t'(z)$. Similarly, let $w_1^\star = \argmin_{z} \sum_{i = t_{j-1}}^{t_j} f_t'(z)$. 

By applying~\Cref{lem:convergence-incremental-gd-shift-lr}, we can show that part B is upper bounded by $\frac{L}{\mu}\sqrt{\frac{2\br{1+\log \Delta_{t_j}} + t_{j-1}D}{\Delta_{t_j}}}$, i.e. 
    
    \begin{equation}\label{eq:second-order-unlearning-B}
        \max_{z\in \cW}\norm{ w_{0, j}^\star - \psi_j'(z)}_2 \leq \frac{L}{\mu}\sqrt{\frac{2\br{1+\log \Delta_{t_j}} + t_{j-1}D}{\Delta_{t_j}}},
    \end{equation}
where $\Delta_{t_j} = t_j - t_{j-1}$. 

Then, we will upper bound part A. To upper bound part A, we only need to upper bound $\norm{H_j(z)\br{\psi_u^{(j)}\circ \psi_j(z) - w_{0, j}^\star}}$. Due to $\mu$-strong convexity of the individual cost functions, $\sum_{t = t_{j-1}}^{t_j} f_t'$ and $\sum_{t = t_{j-1}}^{t_j} f_t$ are both $\Delta_{t_j}\mu$-strongly convex, 
\begin{equation}\label{eq:second-order-unlearning-1}
    \norm{H_j(z)\br{\psi_u^{(j)}\circ \psi_j(z) - w_{0, j}^\star}}\geq \frac{\Delta_{t_j} \mu}{2} \norm{\psi_u^{(j)}\circ \psi_j(z) - w_{0, j}^\star}
\end{equation}

\begin{equation}\label{eq:second-order-unlearning-2}
    \begin{aligned}
     \norm{H_j(z)\br{\psi_u^{(j)}\circ \psi_j(z) - w_{0, j}^\star}} &= \norm{H_j(z)\br{\psi_j(z) - \br{H_j(z)}^{-1} \nabla f_{u_j}(z) - w_{0, j}^\star}}\\
     &= \norm{H_j(z)\br{\psi_j(z) - w_{0, j}^\star} - \nabla f_{u_j}(z)}
    \end{aligned}
\end{equation}

Let $F_1(z) = \sum_{t = t_{j-1}}^{t_j} f_t(z)$ and $F_2(z) = \sum_{t = t_{j-1}}^{t_j} f_t'(z)$. 
\begin{equation}\label{eq:second-order-unlearning-3}
\begin{aligned}
        \norm{  \nabla F_2(\psi_j(z) ) + H_j(z) (w_{0, j}^\star - \psi_j(z))} &\overset{(a)}{=} \norm{\nabla F_2(w_{0, j}^\star)- \nabla F_2(z) - \nabla^2 F_2(\psi_j(z)) (w_{0, j}^\star -\psi_j(z))} \\
        &\leq \frac{\Delta_{t_j}M}{2}\norm{\psi_j(z) - w_{0, j}^\star}^2,
\end{aligned}
\end{equation}
where step (a) follows by the fact that $\nabla F_2(w_{0, j}^\star) = 0$ and the definition of $H_j$. In the last inequality, $M$ is the Hessian Lipschitzness of individual cost functions, obtained by taking Taylor expansion of the function $\nabla F_2(z)$ around the point $w_{0, j}^\star$. 

By definition of $F_1$ and $F_2$, 
\[
     \nabla F_2(\psi_j(z) ) = \nabla F_1(\psi_j(z)) - \nabla f_{u_j}(\psi_j(z) )
\]
Substitute the above equation into~\Cref{eq:second-order-unlearning-3}, we have 
\begin{equation}\label{eq:second-order-unlearning-4}
        \norm{-\nabla f_{u_j}(\psi_j(z)) + H_j(z) (w_{0, j}^\star - \psi_j(z))} \leq \frac{\Delta_{t_j}M}{2}\norm{\psi_j(z) - w_{0, j}^\star}^2 + \norm{\nabla F_1(\psi_j(z)) }
\end{equation}

Next, we combine the previous results, 
\begin{equation}\label{eq:second-order-unlearning-5}
\begin{aligned}
        \norm{\psi_u^{(j)}\circ \psi_j(z) - w_{0, j}^\star} &\overset{(a)}{\leq} \frac{2}{\Delta_{t_j}\mu} \norm{H_j(z)\br{\psi_u^{(j)}\circ \psi_j(z) - w_{0, j}^\star}} \\
        &\overset{(b)}{\leq} \frac{2}{\Delta_{t_j}\mu} \norm{H_j(z)\br{\psi_j(z) - w_{0, j}^\star} - \nabla f_{u_j}(z)}\\
        &\overset{(c)}{\leq} \frac{2}{\Delta_{t_j}\mu} \br{\frac{\Delta_{t_j}M}{2}\norm{\psi_j(z) - w_{0, j}^\star}^2 + \norm{\nabla F_1(\psi_j(z)) }},
\end{aligned}
\end{equation}
where step (a) is due to~\Cref{eq:second-order-unlearning-1}, step (b) is due to~\Cref{eq:second-order-unlearning-2} and step (c) is due to~\Cref{eq:second-order-unlearning-4}. 

By~\Cref{lem:convergence-incremental-gd-shift-lr}, 
\begin{equation}\label{eq:second-order-unlearning-6}
    \norm{\psi_j(z) - w_{0, j}^\star}^2 \leq \frac{2L^2\br{1 + \log \Delta_{t_j}} + t_{j-1}D}{\mu^2\Delta_{t_j}}
\end{equation}
By smoothness of the individual loss function, 
\begin{equation}\label{eq:second-order-unlearning-7}
    \norm{\nabla F_1(\psi_j(z))} = \norm{\nabla F_1(\psi_j(z)) - \nabla F_1(w_{1, j}^\star)} \leq \beta \norm{\psi_j(z) - w_{1, j}^\star} \leq \frac{\beta \Delta_{t_j}}{\mu}\sqrt{\frac{2\br{1 + \log \Delta_{t_j}} + t_{j-1}D}{\Delta_{t_j}}}. 
\end{equation}

Substituting~\Cref{eq:second-order-unlearning-6} and~\Cref{eq:second-order-unlearning-7} into~\Cref{eq:second-order-unlearning-5}, we arrive at an upper bound for Part A
\begin{equation}
    \norm{\psi_u^{(j)}\circ \psi_j(z) - w_{0, j}^\star}\leq \frac{2ML^2 \br{1 + \log \Delta_{t_j}} + t_{j-1}D}{\mu^3\Delta_{t_j}} + \frac{2\beta}{\mu^2}\sqrt{\frac{2\br{1 + \log \Delta_{t_j}} + t_{j-1}D}{\Delta_{t_j}}}. 
\end{equation}

Substituting~\Cref{eq:second-order-unlearning-7} and~\Cref{eq:second-order-unlearning-B} into~\Cref{eq:second-order-unlearning-0}, we arrive at the desired $s_j$, i.e. 
\[s_j \leq  \frac{2ML^2 \br{1 + \log \Delta_{t_j}} + t_{j-1}D}{\mu^3\Delta_{t_j}} + \br{\frac{2\beta}{\mu^2} + \frac{L}{\mu}}\sqrt{\frac{2\br{1 + \log \Delta_{t_j}} + t_{j-1}D}{\Delta_{t_j}}}. \]
\end{proof}

\begin{theorem}\label{thm:second-order-regret}
    Assume all loss functions are $L$-Lipschitz, $\mu$-strongly convex, $\beta$-smooth, and satisfy~\Cref{assump:assumption1}. Assume the set of deletion time satisfies $t_1 \geq \frac{L}{\mu D}$ and $t_i \geq t_{i-1} + e^{Dt_{i-1}}$ for all $i\in [k]$. Assume the index of the unlearning points satisfies $u_i \in (t_{i-1}, t_i)$. Then we can upper bound the regret of the competing algorithm of $\cR_{\cA}^{(2)}$ that unlearns an arbitrary point at time $\cT$ by \[\bE\text{Regret}_T \leq \frac{L^2}{\mu}\br{2 + k(1 + k) +2\log T} + \sum_{i = 1}^k \mu t_i \br{\frac{\varepsilon}{i} + 1}\frac{5i \log \Delta_{t_i}}{\varepsilon\Delta_{t_i}}\br{\frac{5ML^2}{\mu^3} + \frac{2\beta}{\mu^2} + \frac{L}{\mu}}^2.\]
\end{theorem}

\begin{proof}
    The proof is the same as the proof of~\Cref{thm:first-order-regret} until~\Cref{eq:first-order-regret-partB}. 

    Similar to the proof in~\Cref{thm:first-order-regret}, we have that \begin{equation}
        \label{eq:second-order-regret-A}
        \bE\bs{A} \leq \frac{L^2}{\mu}(1 + \log T)
    \end{equation}

    And similarly, following an argument similar to the proof of the unlearning guarnatee for the second order method (\Cref{thm:second-order-unlearning-guarantee}), we can show that $d_i \leq \sigma_i \sqrt{\frac{\varepsilon}{i}}$. Therefore, 
    \begin{equation}
        \label{eq:second-order-regret-B}
        \begin{aligned}
            \bE\bs{B} &\leq d_i (L + \mu t_i D) + \frac{\mu t_i (d_i^2 + \sigma_i^2)}{2} \\
            &\leq \sqrt{\frac{\varepsilon}{i}}\sigma_i\br{L + \mu t_i D} + \frac{\mu t_i \br{\frac{\varepsilon}{i} + 1}\sigma_i^2}{2} \\
            &\leq 2\sqrt{\frac{\varepsilon}{i}}\sigma_i\mu t_i D + \frac{\mu t_i \br{\frac{\varepsilon}{i} + 1}\sigma_i^2}{2} \leq \mu t_i \br{\frac{\varepsilon}{i} + 1}\sigma_i^2
        \end{aligned}
    \end{equation}

    where the last inequality follows by approximation{\color{red}(TODO)}. 

    Next, we show that with some approximation{\color{red} (TODO) }, \begin{equation}
        \label{eq:second-order-sigma2}
        \sigma_i \leq \sqrt{\frac{i}{\varepsilon}}\br{\frac{5ML^2}{\mu^3} + \frac{2\beta}{\mu^2} + \frac{L}{\mu}}\sqrt{\frac{5\log \Delta_{t_i}}{\Delta_{t_i}}}
    \end{equation}

    Substituting~\Cref{eq:second-order-sigma2} into~\Cref{eq:second-order-regret-B} and combine~\Cref{eq:second-order-regret-A,eq:second-order-regret-B}, we have 
    \begin{equation}
        \label{eq:second-order-regret-final}
        \begin{aligned}
            \regret{}{}&\leq \frac{L^2}{\mu}\br{1 + \log T} + \sum_{i = 1}^k \mu t_i \br{\frac{\varepsilon}{i} + 1}\frac{5i \log \Delta_{t_i}}{\varepsilon\Delta_{t_i}}\br{\frac{5ML^2}{\mu^3} + \frac{2\beta}{\mu^2} + \frac{L}{\mu}}^2
        \end{aligned}
    \end{equation}

    Adding the distance between the regret with constant competitor and our regret definition with varying competitor, we complete the proof. 
\end{proof}

\begin{proof}[Proof of~\Cref{lem:FTL-regret1}]
    By induction on $T$: 
    Base case: $T = 1$: $\ell_1 (u) \geq \ell_1(w_2)$ follows by definition of $w_2$. 

    Induction step: known $\sum_{t = 0}^T \ell_t(u)\geq \sum_{t = 0}^T\ell_t(w_{t+1})$, wants to show $\sum_{t = 0}^{T+1} \ell_t(u)\geq \sum_{t = 0}^{T+1}\ell_t(w_{t+1})$. 

    Recall the definition of $w_{T+2} = \text{arg}\min_{w\in \cW}\sum_{t = 1}^{T+1}\ell_t(w)$. 

    Then 
    \begin{equation}
        \begin{aligned}
            \sum_{t = 0}^{T+1} \ell_t (u) &\geq \sum_{t = 0}^{t + 1} \ell_t(x_{T+2})\\
            &= \sum_{t = 1}^T \ell_t(x_{T+2}) +\ell_{T+1}(x_{T+2})\\
            &\geq \sum_{t = 1}^T \ell_t(x_{t+1}) +\ell_{T+1}(x_{T+2})\\
            &= \sum_{t = 1}^{T+1} \ell_t(x_{t+1})
        \end{aligned}
    \end{equation}
    where the inequality follows by the induction hypothesis. 
\end{proof}

\begin{equation}\label{eq:strongly-convex-first-order6}
    \begin{aligned}
        \bE_{\xi_{1:k}}\bs{B} &= \bE\bs{\sum_{i = 1}^k - (\nabla\ell_{t_i-1}(z_{t_i-1}))^\top \xi_i + \frac{\br{z_{t_i - 1}-z^\star}^\top \xi_i + \norm{\xi_i}^2}{2\eta_{t_i-1}}}\\
        &\overset{(a)}{=}\bE\bs{\sum_{i = 1}^k \frac{ \norm{\xi_i}^2}{2\eta_{t_i-1}}} = \sum_{i = 1}^k \frac{\bE\bs{\norm{\xi_i}}^2}{\eta_{t_{i}-1}} \\
        &= \sum_{i = 1}^k \frac{2\mu\br{t_i - 1}(1 + \log \Delta_{t_i})}{\Delta_{t_i}}\br{\frac{\sqrt{2\br{1 + \log \Delta_{t_i}}}ML^2}{\sqrt{\Delta_{t_i}}} + \br{\frac{2\beta + \mu L }{\mu^2}}}^2\\
        &\overset{(b)}{\leq}  \frac{2.2\br{4\beta^2 + 4\beta \mu L + \mu^2 L^2}}{\mu^3}\sum_{i = 1}^k  \frac{\br{t_i - 1}\br{1 + \log \Delta_{t_i}}}{\Delta_{t_i}}
    \end{aligned}   
\end{equation}

where step (b) follows by the assumption that $\Delta_{t_i}$ satisfy $\frac{ML^2\sqrt{2\br{1 + \log \Delta_{t_i}}}}{\sqrt{\Delta_{t_i}}}\leq \frac{2\beta + L \mu}{5\mu^2}$.
