# Supplementary material for: Online Learning and Unlearning
Source: arXiv:2505.08557 source file (2025-05-13)
Supplement: Supplementary file 5 [file general-unlearning.tex]

\begin{algorithm}[htbp]
    \caption{General active online learner and unlearner}
    \label{alg:general-active}
    \begin{algorithmic}[1]
        \REQUIRE Cost functions $f_1, ..., f_T$ that are $L$-Lipschitz, learning rates $\eta_1, ..., \eta_T$, a deletion time set $\cT$, a deletion index set $\cU$, and privacy parameter $\varepsilon$, the auxiliary unlearner $\Unaux$ and its Lipschitz parameter $L_R$ and error functions $e_2, e_1$. 
        \STATE Initialize $z_1\in \cK$. 
        \FOR{Time step $t = 2, ... T$}
            \STATE Set $z_t = z_{t-1} - \eta_t \nabla f_{t-1}(z_{t-1})$
            \IF{there exists $t_i\in \cT$ such that $t = t_i$}
            \STATE Set $z_{t_i} = \Unaux(z_t, \{f_{u_j}\}_{j = 1}^i, f_{1:{t_i}}) + \xi_i$, where $\xi_i \sim \cN(0, \sigma_i^2)$ for 
            \begin{equation}
                \label{eq:sigma-i-active}\sigma_i = \sqrt{\frac{\alpha j^\omega \omega}{2(\omega -1)\varepsilon}}\br{\max_{z\in \cK}\norm{\Unaux(z, \trainsetsub{t_j}, \unlearnsetsub{j}) - \Unaux(z, \trainsetsub{t_j}\setminus \unlearnsetsub{j},\emptyset )}_2 + L_R \gamma^{t_i - u_i}\eta_{u_i}L}.
            \end{equation}
            \COMMENT{$\mathtt{\Unaux^{(1)}}(z, \mathtt{f_{u_i}}, \mathtt{f_{1:t}})$ applies $\cI_1$ gradient descent steps with $\mathtt{f_{1:t_i}}$ and $\cI_2$ gradient descent steps with $\mathtt{f_{1:t_i}}\setminus \{\mathtt{f_{u_j}}\}_{j = 1}^i$}
        \ENDIF
        \STATE Output $z_t$ 
        \ENDFOR
    \end{algorithmic}
\end{algorithm}

% \ActiveGeneral*
\begin{proof}[Unlearning guarantee]
    Up until the ith deletion, we first write the two CNIs. For $\cF = \{f_1, ..., f_{t_i}\}$ and $\cF' = \cF$ with points at $u_j$, $j\leq i$ replaced with $\perp$. 

    Then, $\psi_j$ denote the gradient descent steps between $t_{j-1}$ and $t_j$ using points in $\cF$, i.e. for updating function $g_t$ and $g_t'$ with respect to $\cF$ and $\cF'$ respectively, 
    \[\psi_j = g_{t_{j}}\circ\ldots \circ g_{t_{j-1}}, \quad \psi_j' = g_{t_{j}}'\circ\ldots \circ g_{t_{j-1}}' \]
    Then, the CNIs are 
    \[\bc{z_0, \bc{\Unaux(\psi_j, \trainsetsub{t_i}, \unlearnsetsub{i})}_{j = 1}^i, \bc{\zeta_j}_{j = 1}^i}, \quad \bc{z_0, \bc{\Unaux(\psi_j', \trainsetsub{t_i}\setminus \unlearnsetsub{i},\emptyset )}_{j = 1}^i, \bc{\zeta_j}_{j = 1}^i}\]
    Therefore, we need to upper bound, for all $j\in [i]$,
    \begin{equation}
        \begin{aligned}
            s_j &= \max_{z\in \cK}\norm{\Unaux(\psi_j(z), \trainsetsub{t_j}, \unlearnsetsub{j}) - \Unaux(\psi_j'(z), \trainsetsub{t_j}\setminus \unlearnsetsub{j},\emptyset )}_2
        \end{aligned}
    \end{equation}

   As we assume $u_i \in (t_{i-1}, t_i)$ for all $i$, 
   \begin{equation}\small
    \begin{aligned}
        s_j &= \max_{z\in \cK}\norm{\Unaux(\psi_j(z), \trainsetsub{t_j}, \unlearnsetsub{j}) - \Unaux(\psi_j'(z), \trainsetsub{t_j}\setminus \unlearnsetsub{j},\emptyset )}_2\\
        &= \max_{z\in \cK}\norm{\Unaux(\psi_j(z), \trainsetsub{t_j}, \unlearnsetsub{j}) - \Unaux(\psi_j(z), \trainsetsub{t_j}\setminus \unlearnsetsub{j},\emptyset ) + \Unaux(\psi_j(z), \trainsetsub{t_j}\setminus \unlearnsetsub{j},\emptyset ) - \Unaux(\psi_j'(z), \trainsetsub{t_j}\setminus \unlearnsetsub{j},\emptyset )}_2\\
        &= \max_{z\in \cK}\norm{\Unaux(z, \trainsetsub{t_j}, \unlearnsetsub{j}) - \Unaux(z, \trainsetsub{t_j}\setminus \unlearnsetsub{j},\emptyset )}_2 + L_R(\psi_j(z) - \psi_j(z)')\\
        & =\max_{z\in \cK}\norm{\Unaux(\psi_j(z), \trainsetsub{t_j}, \unlearnsetsub{j}) - \Unaux(\psi_j(z), \trainsetsub{t_j}\setminus \unlearnsetsub{j},\emptyset )}_2 + L_R \gamma^{t_i - u_i}\eta_{u_i}L
    \end{aligned}
   \end{equation}
    where $L_R$ is the Lipschitzness coefficient of the unlearning algorithm $\Unaux$. 
   
   Setting $a_i = s_i$ and $\sigma^2 = \frac{\alpha\omega j^\omega a_i^2}{2(\omega -1)\varepsilon}$, we have the following guarantee: for all $i\in [k]$, \[\rdp{z_{t_i}}{z_{t_i}'}\leq \sum_{j = 1}^i R(\zeta_{t_i}, a_i) \leq \varepsilon. \]
\end{proof}

\begin{proof}
    Following a similar argument as in the previous section, for any $z^\star$, for $i\in [k]$, the regret between $t_i$ to $t_{i+1}$ is upper bounded by the regret of running OGD on cost functions $f_{t_i}:f_{t_{i+1}}$ with initialization $z_{t_i} = \Unaux\br{\hat{z}_{t_i}, f_{1:t_{i}}, f_{u_1:u_i}} + \xi_i$ where $\hat{z}_{t_i}$ is obtained by one gradient descent step on $z_{t_{i-1}}$ and $\xi_i$ is sampled from according to~\Cref{alg:active-general}. We note that this regret is upper bounded by the regret bound of OGD with arbitrary initializations. Therefore, the final regret is upper bounded by $\sum_{i = 1}^k \frac{L^2}{\mu}(1 + \log T) \leq \frac{kL^2}{\mu}\br{1 + \log T}$. 
\end{proof}
